# Supplementary material for: Deep Learning-Driven Prediction of Microstructure Evolution via Latent Space Interpolation
Source: arXiv:2508.01822 ancillary file (2025-08-03)
Supplement: Supplementary file 1 [file anc.pdf]

# Supplementary Material
# Deep Learning-Driven Prediction of Microstructure Evolution via Latent Space Interpolation*

Sachin Gaikwad,[1,†] Thejas Kasilingam,[2,†] Owais Ahmad,[2] Rajdip Mukherjee,[2] and Somnath Bhowmick[2,‡]

[1]*School of Materials Science and Technology, Indian Institute of Technology (BHU), Varanasi, India*

[2]*Department of Materials Science & Engineering, Indian Institute of Technology, Kanpur, Kanpur 208016, India*

(Dated: August 3, 2025)

The supplementary material contains generated microstructures over the entire composition range of $c_{avg} = 0.27$ to 0.48.

* Code available on GitHub.

† These authors contributed equally to this work.

‡ bsomnath@iitk.ac.in

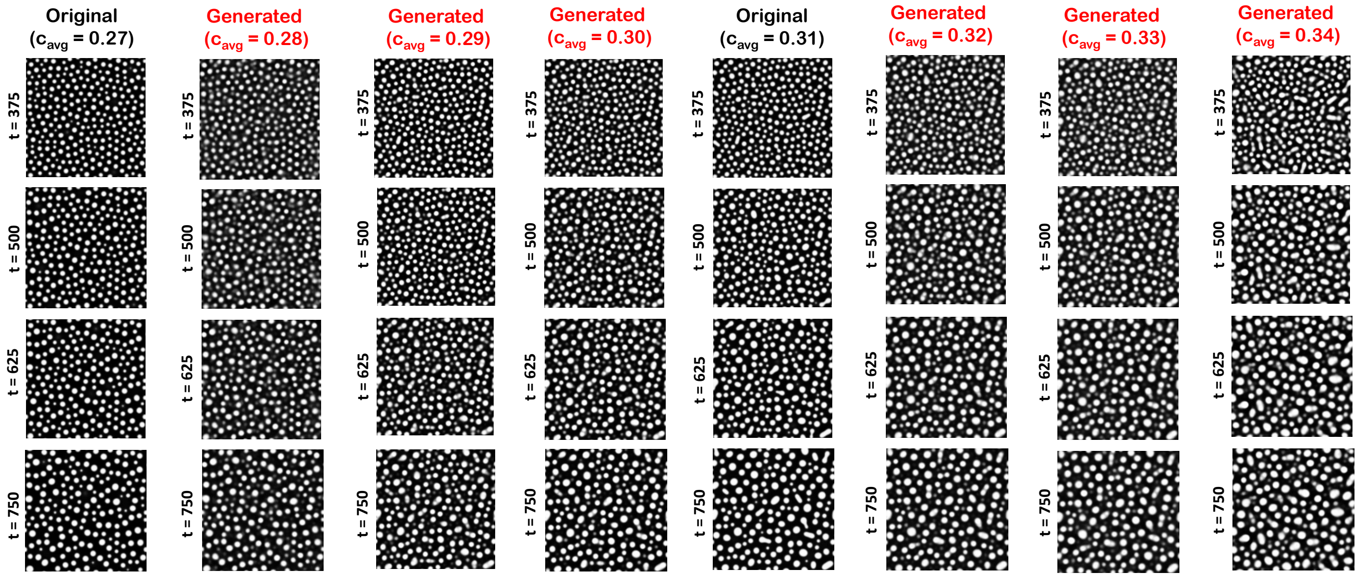


FIG. S1. Comparison of original and CVAE-generated microstructure evolution for composition interval 0.27 → 0.34.

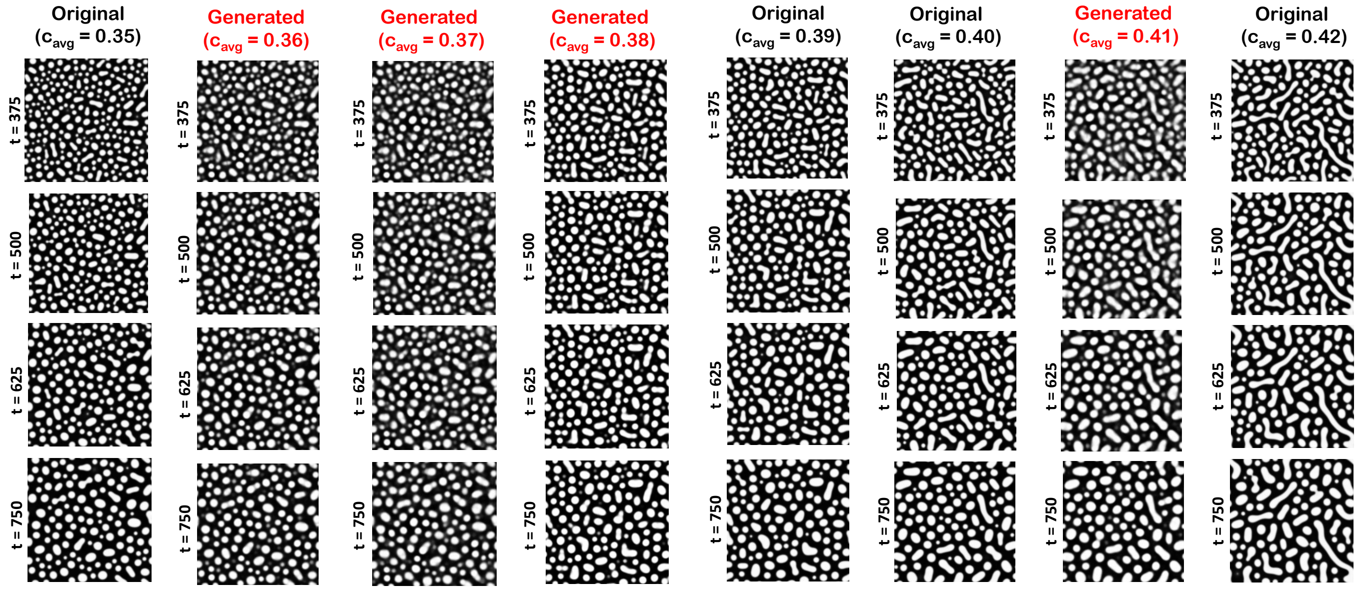


FIG. S2. Comparison of original and CVAE-generated microstructure evolution for composition interval 0.35 → 0.42.

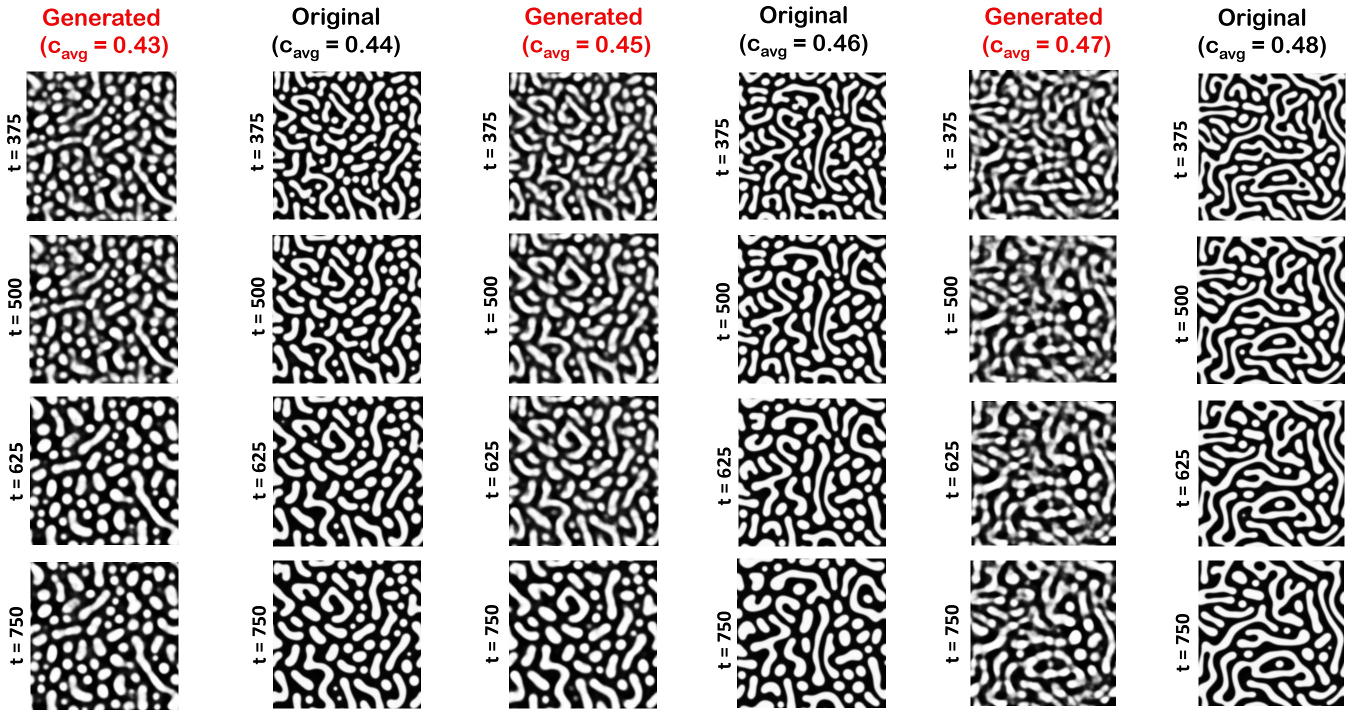


FIG. S3. Comparison of original and CVAE-generated microstructure evolution for composition interval 0.43 → 0.48.
